# Supplementary material for: Personalized Image Generation for Recommendations Beyond Catalogs
Source: arXiv:2502.18477 source file (2025-11-25)
Supplement: Supplementary file 1 [file X_suppl.tex]

\clearpage
\setcounter{page}{1}
\maketitlesupplementary

\section{Rationale}
\label{sec:rationale}
Having the supplementary compiled together with the main paper means that:
\begin{itemize}
\item The supplementary can back-reference sections of the main paper, for example, we can refer to \cref{sec:intro};
\item The main paper can forward reference sub-sections within the supplementary explicitly (e.g. referring to a particular experiment); 
\item When submitted to arXiv, the supplementary will already included at the end of the paper.
\end{itemize}
To split the supplementary pages from the main paper, you can use \href{https://support.apple.com/en-ca/guide/preview/prvw11793/mac#:~:text=Delete%20a%20page%20from%20a,or%20choose%20Edit%20%3E%20Delete).}{Preview (on macOS)}, \href{https://www.adobe.com/acrobat/how-to/delete-pages-from-pdf.html#:~:text=Choose%20%E2%80%9CTools%E2%80%9D%20%3E%20%E2%80%9COrganize,or%20pages%20from%20the%20file.}{Adobe Acrobat} (on all OSs), as well as \href{https://superuser.com/questions/517986/is-it-possible-to-delete-some-pages-of-a-pdf-document}{command line tools}.

\section{LoRA per User}
\label{suppl:lpu}
\begin{table}[t]
\centering
\small
\setlength{\tabcolsep}{6pt}

\caption{\textbf{Per-user LoRA training hyperparameters.} The LoRA rank ($r$), scaling factor ($\alpha$), dropout, training steps, and warmup schedule are adapted based on the number of available user images ($N_i$).}
\label{tab:lora_hyperparams}
\begin{tabular}{c c c c c c}
\toprule
\textbf{$N_i$ range} & \textbf{LoRA $r$} & \textbf{LoRA $\alpha$} & \textbf{Dropout} & \textbf{Steps} & \textbf{Warmup} \\
\midrule
$N_i < 8$           & 8  & 8  & 0.10 & 1200 & 100  \\
$8 \le N_i \le 24$  & 16 & 16 & 0.07 & 1500 & 120  \\
$25 \le N_i \le 60$ & 32 & 32 & 0.05 & 1700 & 150  \\
$61 \le N_i \le 120$& 64 & 64 & 0.05 & 2000 & 200  \\
$N_i > 120$         & 32 & 32 & 0.05 & 2500 & 200  \\
\bottomrule
\end{tabular}
\end{table}

\section{Ablations}
\subsection{}
